# Supplementary material for: Architectural Neural Backdoors from First Principles
Source: arXiv:2402.06957 source file (2024-02-10)
Supplement: Supplementary file 1 [file additional.tex]

\section{Additional}

Additional things we looked at were:

\begin{itemize}

\item Whether hypernetworks overfit more -- we hypothesise that they do. This poses a potential data-as-code attack threat.

\end{itemize}
